# Supplementary material for: Computation of Singular Godeaux Surfaces and a New Explicit Fake Quadric (With an Appendix by Christian Gleissner and Noah Ruhland)
Source: arXiv:2509.08198 ancillary file (2026-07-10)
Supplement: Supplementary file 1 [file Main_with_output.pdf]

```

1  Magma V2.28-27    Wed Sep  3 2025 22:18:14 on bomb      [Seed = 2759097425]
2  Type ? for help.  Type <Ctrl>-D to quit.
3  >
4  > // This is an arXiv ancillary file for the paper
5  > // 'Computation of Singular Godeaux Surfaces and a New Explicit Fake Quadric',
6  > // by Carlos Rito.
7  >
8  > // We give equations of a surface Y with an involution i acting.
9  > // The first goal is to show that Y is a surface with  $p_g=1$ ,  $q=0$ ,  $K^2=2$ ,
10 > // with singular set  $4A_3+4A_1$ , and the involution acts freely
11 > // (so  $X:=Y/i$  is a numerical Godeaux surface with singular set  $2A_3+2A_1$ ).
12 >
13 > // We start by defining Y over a quadratic extension of the rationals.
14 >
15 > SetNthreads(16);
16 >
17 > K:=Rationals();
18 > R<e>:=PolynomialRing(K);
19 > K<e>:=ext<K|e^2-2765569/233280>;
20 > R8<x0,x1,x2,x3,x4,x5,x6,x7>:=PolynomialRing(K,8,"grevlex");
21 > P7:=ProjectiveSpace(R8);
22 >
23 > // We load the surface Y:
24 > load "Eqs_of_Y_and_singularities.txt";
25 Loading "Eqs_of_Y_and_singularities.txt"
26 > Y:=Surface(P7,Eqs);
27 >
28 > // Y is invariant for the involution i in  $P^7$ :
29 > Y eq Scheme(P7,[Evaluate(q,[x0,x1,-x2,-x3,x4,x5,-x6,-x7]):q in Eqs]);
30 true
31 >
32 > // And the involution acts freely:
33 > Dimension(Scheme(Y,[x2,x3,x6,x7])) eq -1;
34 true
35 > Dimension(Scheme(Y,[x0,x1,x4,x5])) eq -1;
36 true
37 >
38 > // We also load defining equations of 8 points that
39 > // we show are singular points of Y:
40 > singY:=&cat[Setseq(Points(Scheme(P7,q))):q in pc];
41 > #singY eq 8;
42 true
43 > &and[IsSingular(Y,q):q in singY];
44 true
45 >
46 > // We will show below that Y has no other singularities
47 > // (computing over a finite field).
48 >
49 > // Now we define a map  $Y \rightarrow P^3$  that we show is birational:
50 > P3:=ProjectiveSpace(K,3);
51 > phi:=map<Y->P3|[x0,x1,x2,x3]>;
52 >
53 > // We know that Y is embedded in  $P^7$  by its 3-canonical map
54 > // (see J. Algebr. Geom. 31, No. 1, 127-135 (2022)).
55 > // In fact we show that the canonical divisor is:
56 > KY:=Scheme(Y,[x0,x1,x2,x3]);
57 >
58 > // Confirmation (this takes 1h or more):
59 > // KY eq Scheme(P7,Basis(Ideal(CanonicalDivisor(Y))));
60 >

```

```

61 > // And there is an hyperplane that cuts Y at KY with multiplicity 3:
62 > H:=Scheme(Y,x0);
63 > H:=Difference(H,KY);
64 > KY eq Difference(H,KY);
65 true
66 >
67 > // From
68 > Degree(Y) eq 18;
69 true
70 > // we get  $(3K_Y)^2=18$ , thus  $K_Y^2=2$ .
71 >
72 > // Since KY is the base scheme of phi,
73 > // we conclude that phi is the bicanonical map of Y.
74 >
75 > // Now phi sends Y to an octic surface:
76 > O:=phi(Y);
77 > Degree(O) eq 8;
78 true
79 > // And since  $(2K_Y)^2=8$ , then phi is birational.
80 >
81 > // Notice that the base scheme of phi is KY.
82 > // The map phi is defined on the 8 singularities:
83 > &or[q in KY:q in singY] eq false;
84 true
85 >
86 > // It is faster to study the singularities on the bicanonical image of Y.
87 > // We map those 8 points to singularities of the octic O:
88 > singO:=[phi(q):q in singY];
89 > #Seqset(singO) eq 8;
90 true
91 >
92 > // These points are disjoint from the codimension 1 singular subvariety of O.
93 > // We show they are of type  $A_3, A_3, A_3, A_3, A_1, A_1, A_1, A_1$ :
94 > for q in singO do IsSimpleSurfaceSingularity(O!q);end for;
95 true A 3
96 true A 3
97 true A 3
98 true A 3
99 true A 1
100 true A 1
101 true A 1
102 true A 1
103 >
104 > // The pullback of each of these 8 points is one single point in Y
105 > // (we remove the base scheme of phi),
106 > // thus Y also has 8 singularities of the same type:
107 > for q in singO do
108 for> Pb:=Pullback(phi,q);
109 for> Pb:=Difference(Pb,B);
110 for> [Dimension(Pb),Degree(Pb)] eq [0,1];
111 for> end for;
112 true
113 true
114 true
115 true
116 true
117 true
118 true
119 true
120 >

```

```

121 > // We still have to show that Y has no other singularities,
122 > // but this is shown easily working over finite fields, see below.
123 >
124 > // Below we do computations with the curve D,
125 > // but let us show here that D contains two A_3 and the four A_1 singularities
126 > // (the reason for doing it here is that below we are not considering the above
127 > // quadratic extension that is needed to define the singularities).
128 > load "Eqs_of_D.txt";
129 Loading "Eqs_of_D.txt"
130 > D:=Scheme(P7,Eqs);
131 > [pt in D:pt in singY];
132 [ false, false, true, true, true, true, true, true ]
133 >
134 >
135 > //////////////////////////////////////
136 >
137 >
138 > // We do some computations with the curve D, over the rational field:
139 >
140 > SetNthreads(16);
141 >
142 > K:=Rationals();
143 > R8<x0,x1,x2,x3,x4,x5,x6,x7>:=PolynomialRing(K,8,"grevlex");
144 > P7:=ProjectiveSpace(R8);
145 >
146 > load "Eqs_of_Y_and_singularities.txt";
147 Loading "Eqs_of_Y_and_singularities.txt"
148 > Y:=Surface(P7,Eqs);
149 > KY:=Scheme(Y,[x0,x1,x2,x3]);
150 >
151 > load "Eqs_of_D.txt";
152 Loading "Eqs_of_D.txt"
153 > D:=Scheme(P7,Eqs);
154 >
155 > // D is invariant for the involution:
156 > D eq Scheme(P7,[Evaluate(q,[x0,x1,-x2,-x3,x4,x5,-x6,-x7]):q in Eqs]);
157 true
158 >
159 > // And D is smooth:
160 > SD:=SingularSubscheme(D);
161 > Dimension(SD) eq -1;
162 true
163 >
164 > //We show that there is an element in the linear system |4K_Y|
165 > // which is invariant for the involution and cuts Y at 2D.
166 >
167 > // A certain element in |6K_Y|:
168 > f:=-3239913*x1^2-3466925*x2*x3+3743007*x0*x4+70338*x1*x4+2715*x4^2-24687*x0*x5+
169 > 2715*x4*x5+89847*x2*x6+2715*x3*x6-103422*x2*x7+10860*x3*x7+2715*x6*x7-2715*x7^2;
170 > D2:=Scheme(Y,f);
171 > Degree(D2) eq 36;
172 true
173 >
174 > // We remove K_Y two times:
175 > D2:=Difference(D2,KY);
176 > D2:=Difference(D2,KY);
177 > Degree(D2) eq 24;
178 true
179 >
180 > // Let's see that D2 is D with multiplicity 2:

```

```

181 > D eq Difference(D2,D);
182 true
183 >
184 > // To see that D is irreducible, we can do:
185 > // C:=Curve(P7,DefiningEquations(D));
186 > // IsAbsolutelyIrreducible(C);
187 > // It is enough and much faster to do it over a finite field.
188 >
189 >
190 > //////////////////////////////////////
191 >
192 >
193 > // Now to speed-up computations, we work over a finite field:
194 > p:=1589683;K:=GF(p);
195 >
196 > // To define the curve C below, we need a quadratic extension of K:
197 > R<r>:=PolynomialRing(K);
198 > load "The_quadratic_Extension.txt";
199 Loading "The_quadratic_Extension.txt"
200 > K<r>:=ext<K|Normalize(f)>;
201 >
202 > R8<x0,x1,x2,x3,x4,x5,x6,x7>:=PolynomialRing(K,8,"grevlex");
203 > P7:=ProjectiveSpace(R8);
204 >
205 > // We load again the equations of the surface Y:
206 > load "Eqs_of_Y_and_singularities.txt";
207 Loading "Eqs_of_Y_and_singularities.txt"
208 > Y:=Surface(P7,Eqs);
209 > KY:=Scheme(Y,[x0,x1,x2,x3]);
210 >
211 > // And we finally show that Y has exactly the above 8 singular points:
212 > SY:=ReducedSubscheme(SingularSubscheme(Y));
213 > Dimension(SY) eq 0;
214 true
215 > Degree(SY) eq 8;
216 true
217 >
218 > // The singularities of Y are:
219 > singY:=&cat[Setseq(Points(Scheme(P7,q))):q in pc];
220 > #singY eq 8;
221 true
222 >
223 > // We have shown that all singularities of Y are rational double points.
224 >
225 > // Now we compute the number of connected components of Y,
226 > // the irregularity q and the geometric genus p_g.
227 > // Notice that, by semicontinuity, cohomology can only go up
228 > // when computed over a finite field.
229 >
230 > I:=Ideal(Y);
231 > O_X:=GradedModule(I);
232 >
233 > //  $h^0(X,O_X)=1$ , thus X is connected:
234 > CohomologyDimension(O_X,0,0) eq 1;
235 true
236 >
237 > // Irregularity q=0:
238 > CohomologyDimension(O_X,1,0) eq 0;
239 true
240 >

```

```

241 > // GeometricGenus p_g=1:
242 > CohomologyDimension(0_X,2,0) eq 1;
243 true
244 >
245 > // We note that if p_g=0 (over the rationals), then the holomorphic Euler characteristic
246 > // would be \chi=1, which is impossible because since Y has a fixed point free
247 > // involution, \chi must be even (double of the quotient).
248 >
249 > // We check again that K_Y^2=2:
250 > KD:=CanonicalDivisor(Y);
251 > SelfIntersection(KD) eq 2;
252 true
253 >
254 >
255 > //////////////////////////////////////
    //////////////////////////////////
256 >
257 >
258 > // Some computations with the curve C:
259 >
260 > load "Eqs_of_C_and_4C.txt";
261 Loading "Eqs_of_C_and_4C.txt"
262 > C:=Curve(P7,Eqs);
263 > C subset Y;
264 true
265 > Degree(C) eq 12;
266 true
267 >
268 > // C is invariant for the involution:
269 > {q div Evaluate(q,[x0,x1,-x2,-x3,x4,x5,-x6,-x7]):q in Eqs} eq {-1,1};
270 true
271 >
272 > // C is irreducible.
273 > IsAbsolutelyIrreducible(C);
274 true
275 >
276 > // And C is smooth:
277 > SC:=SingularSubscheme(C);
278 > Dimension(SC) eq -1;
279 true
280 >
281 > // C contains the four A_3 and two A_1:
282 > [pt in C:pt in singY];
283 [ true, true, true, true, false, false, true, true ]
284 >
285 > // Now we show that there is an element in the linear system |8K_Y|
286 > // which is invariant for the involution and cuts Y at 4C.
287 >
288 > // We have loaded a certain degree 3 polynomial F:
289 > Type(F) eq RngMPolElt, Degree(F) eq 3;
290 true true
291 >
292 > // It is invariant for the involution:
293 > F eq Evaluate(F,[x0,x1,-x2,-x3,x4,x5,-x6,-x7]);
294 true
295 >
296 > // It cuts a scheme in Y that contains the canonical divisor K_Y:
297 > C4:=Scheme(Y,F);
298 > IsSubscheme(KY,C4);
299 true

```

```
300 >
301 > // We remove it:
302 > C4:=Difference(C4,KY);
303 > // So now C4 is in |8K_Y|.
304 >
305 > // We want to show that C4 is C with multiplicity 4.
306 > // To speed-up computations, we work on the (birational)
307 > // bicanonical image of Y.
308 >
309 > // The bicanonical map:
310 > P3:=ProjectiveSpace(K,3);
311 > phi:=map<P7->P3| [x0,x1,x2,x3]>;
312 >
313 > // The images of C and C4:
314 > phiC:=phi(C);
315 > phiC4:=phi(C4);
316 >
317 > // If the support of C4 is not the (irreducible) curve C,
318 > // then C4 has at least one more irreducible component.
319 > // This is not the case:
320 > IsEmpty(Complement(phiC4,phiC));
321 true
322 >
323 > // Since
324 > Degree(C4) eq 4*Degree(C);
325 true
326 > // then C4=4*C;
327 >
328 > // REMARK: These computations showing that C4=4*C must be done over
329 > // characteristic zero:
330 > // We take K:=Rationals() instead of K:=GF(p) above.
331 > // But this takes long!
```
